# Supplementary material for: On the Robustness of Deep Clustering Models: Adversarial Attacks and Defenses
Source: arXiv:2210.01940 source file (2022-10-04)
Supplement: Supplementary file 1 [file appendix.tex]

% For APPENDIX please view non-arxiv version in Overleaf.
